# Supplementary material for: REINFOREST: Reinforcing Semantic Code Similarity for Cross-Lingual Code Search Models
Source: arXiv:2305.03843 source file (2024-04-15)
Supplement: Supplementary file 1 [file main.tex]

\begin{table*}[h]
\centering
\caption{\textbf{Detailed Results of Searching Python Code with Java Code as query}}
\label{tab:java_res}
% \resizebox{\textwidth}{!}
{%
\begin{tabular}{ccccc|ccccccc}
\hlineB{2}
\multicolumn{5}{c|}{\textbf{Settings}} & \multicolumn{7}{c}{\textbf{Metrics}} \bigstrut \\ \hlineB{2}
\multicolumn{1}{c|}{\textbf{Model}} & \multicolumn{1}{c|}{\textbf{Sub-Model}} & \multicolumn{1}{c|}{\textbf{Trained}} & \multicolumn{1}{c|}{\textbf{SSS}} & $\mathbf{\alpha}$ & \multicolumn{1}{c|}{\textbf{PR@1}} & \multicolumn{1}{c|}{\textbf{PR@2}} & \multicolumn{1}{c|}{\textbf{PR@3}} & \multicolumn{1}{c|}{\textbf{PR@4}} & \multicolumn{1}{c|}{\textbf{PR@5}} & \multicolumn{1}{c|}{\textbf{AFP}} & \textbf{ARG} \bigstrut \\ \hlineB{2}
\multicolumn{1}{c|}{BM25} & \multicolumn{4}{c|}{\cellcolor[HTML]{FFFFFF}} & \multicolumn{1}{c|}{15.14} & \multicolumn{1}{c|}{13.56} & \multicolumn{1}{c|}{12.25} & \multicolumn{1}{c|}{11.59} & \multicolumn{1}{c|}{11.17} & \multicolumn{1}{c|}{48.93} & 0.1209 \bigstrut \\ \cline{1-1} \cline{6-12} 
\multicolumn{1}{c|}{Token-Subset (COSAL)} & \multicolumn{4}{c|}{\cellcolor[HTML]{FFFFFF}} & \multicolumn{1}{c|}{59.76} & \multicolumn{1}{c|}{57.95} & \multicolumn{1}{c|}{56.08} & \multicolumn{1}{c|}{54.79} & \multicolumn{1}{c|}{53.73} & \multicolumn{1}{c|}{20.71} & 0.2496 \bigstrut \\ \cline{1-1} \cline{6-12} 
\multicolumn{1}{c|}{Tree-Similarity (stratified)} & \multicolumn{4}{c|}{\multirow{-3}{*}{\cellcolor[HTML]{FFFFFF}No-Training   required}} & \multicolumn{1}{c|}{53.33} & \multicolumn{1}{c|}{48.33} & \multicolumn{1}{c|}{47.04} & \multicolumn{1}{c|}{45.28} & \multicolumn{1}{c|}{43.11} & \multicolumn{1}{c|}{17.03} & 0.23336 \bigstrut \\ \hlineB{2}
\multicolumn{1}{c|}{} & \multicolumn{4}{c|}{CodeBERT  (stratified)} & \multicolumn{1}{c|}{29} & \multicolumn{1}{c|}{29} & \multicolumn{1}{c|}{29.17} & \multicolumn{1}{c|}{29} & \multicolumn{1}{c|}{29.5} & \multicolumn{1}{c|}{22.88} & 0.2947 \bigstrut \\ \cline{2-12} 
\multicolumn{1}{c|}{} & \multicolumn{4}{c|}{GraphCodeBERT    (stratified)} & \multicolumn{1}{c|}{13.5} & \multicolumn{1}{c|}{10.5} & \multicolumn{1}{c|}{10.67} & \multicolumn{1}{c|}{11.63} & \multicolumn{1}{c|}{11.9} & \multicolumn{1}{c|}{59.98} & 0.2814 \bigstrut \\ \cline{2-12} 
\multicolumn{1}{c|}{\multirow{-3}{*}{Single-Encoder   Models}} & \multicolumn{4}{c|}{UnixCoder  (stratified)} & \multicolumn{1}{c|}{61.5} & \multicolumn{1}{c|}{60} & \multicolumn{1}{c|}{62} & \multicolumn{1}{c|}{63} & \multicolumn{1}{c|}{63.4} & \multicolumn{1}{c|}{8.33} & 0.3559 \bigstrut \\ \hlineB{2}
\multicolumn{1}{c|}{} & \multicolumn{1}{c|}{\cellcolor[HTML]{F8D8D8}-} & \multicolumn{1}{c|}{\cellcolor[HTML]{F8D8D8}N} & \multicolumn{1}{c|}{\cellcolor[HTML]{F8D8D8}-} & \cellcolor[HTML]{F8D8D8}- & \multicolumn{1}{c|}{\cellcolor[HTML]{F8D8D8}10.5} & \multicolumn{1}{c|}{\cellcolor[HTML]{F8D8D8}10.06} & \multicolumn{1}{c|}{\cellcolor[HTML]{F8D8D8}9.73} & \multicolumn{1}{c|}{\cellcolor[HTML]{F8D8D8}9.7} & \multicolumn{1}{c|}{\cellcolor[HTML]{F8D8D8}9.42} & \multicolumn{1}{c|}{\cellcolor[HTML]{F8D8D8}48.95} & \cellcolor[HTML]{F8D8D8}0.0871 \bigstrut \\ \cline{2-12} 
\multicolumn{1}{c|}{} & \multicolumn{1}{c|}{\cellcolor[HTML]{FCE5CD}-} & \multicolumn{1}{c|}{\cellcolor[HTML]{FCE5CD}Y} & \multicolumn{1}{c|}{\cellcolor[HTML]{FCE5CD}N} & \cellcolor[HTML]{FCE5CD}0 & \multicolumn{1}{c|}{\cellcolor[HTML]{FCE5CD}80.77} & \multicolumn{1}{c|}{\cellcolor[HTML]{FCE5CD}79.55} & \multicolumn{1}{c|}{\cellcolor[HTML]{FCE5CD}78.44} & \multicolumn{1}{c|}{\cellcolor[HTML]{FCE5CD}77.02} & \multicolumn{1}{c|}{\cellcolor[HTML]{FCE5CD}75.22} & \multicolumn{1}{c|}{\cellcolor[HTML]{FCE5CD}13.79} & \cellcolor[HTML]{FCE5CD}0.3407 \bigstrut \\ \cline{2-12} 
\multicolumn{1}{c|}{\multirow{-3}{*}{CodeBERT}} & \multicolumn{1}{c|}{\cellcolor[HTML]{D9EAD3}{\color[HTML]{00009B} \textbf{-}}} & \multicolumn{1}{c|}{\cellcolor[HTML]{D9EAD3}{\color[HTML]{00009B} \textbf{Y}}} & \multicolumn{1}{c|}{\cellcolor[HTML]{D9EAD3}{\color[HTML]{00009B} \textbf{Y}}} & \cellcolor[HTML]{D9EAD3}{\color[HTML]{00009B} \textbf{0.2}} & \multicolumn{1}{c|}{\cellcolor[HTML]{00FF00}{\color[HTML]{00009B} \textbf{86.47}}} & \multicolumn{1}{c|}{\cellcolor[HTML]{00FF00}{\color[HTML]{00009B} \textbf{85.46}}} & \multicolumn{1}{c|}{\cellcolor[HTML]{00FF00}{\color[HTML]{00009B} \textbf{84.77}}} & \multicolumn{1}{c|}{\cellcolor[HTML]{00FF00}{\color[HTML]{00009B} \textbf{83.77}}} & \multicolumn{1}{c|}{\cellcolor[HTML]{00FF00}{\color[HTML]{00009B} \textbf{82.62}}} & \multicolumn{1}{c|}{\cellcolor[HTML]{00FF00}{\color[HTML]{00009B} \textbf{9.53}}} & \cellcolor[HTML]{00FF00}{\color[HTML]{00009B} \textbf{0.3857}} \bigstrut \\ \hlineB{2}
\multicolumn{1}{c|}{} & \multicolumn{1}{c|}{} & \multicolumn{1}{c|}{\cellcolor[HTML]{F8D8D8}N} & \multicolumn{1}{c|}{\cellcolor[HTML]{F8D8D8}-} & \cellcolor[HTML]{F8D8D8}- & \multicolumn{1}{c|}{\cellcolor[HTML]{F8D8D8}34.07} & \multicolumn{1}{c|}{\cellcolor[HTML]{F8D8D8}32.99} & \multicolumn{1}{c|}{\cellcolor[HTML]{F8D8D8}32.23} & \multicolumn{1}{c|}{\cellcolor[HTML]{F8D8D8}31.94} & \multicolumn{1}{c|}{\cellcolor[HTML]{F8D8D8}31.55} & \multicolumn{1}{c|}{\cellcolor[HTML]{F8D8D8}19.69} & \cellcolor[HTML]{F8D8D8}0.1907 \bigstrut \\ \cline{3-12} 
\multicolumn{1}{c|}{} & \multicolumn{1}{c|}{} & \multicolumn{1}{c|}{Y} & \multicolumn{1}{c|}{N} & 0 & \multicolumn{1}{c|}{64.45} & \multicolumn{1}{c|}{63.74} & \multicolumn{1}{c|}{62.75} & \multicolumn{1}{c|}{62.06} & \multicolumn{1}{c|}{61.46} & \multicolumn{1}{c|}{11.87} & 0.3442 \bigstrut \\ \cline{3-12} 
\multicolumn{1}{c|}{} & \multicolumn{1}{c|}{\multirow{-3}{*}{Ada}} & \multicolumn{1}{c|}{Y} & \multicolumn{1}{c|}{Y} & 0.2 & \multicolumn{1}{c|}{66.77} & \multicolumn{1}{c|}{65.85} & \multicolumn{1}{c|}{65.24} & \multicolumn{1}{c|}{64.58} & \multicolumn{1}{c|}{63.81} & \multicolumn{1}{c|}{10.6} & 0.3458 \bigstrut \\ \clineB{2-12}{2}
\multicolumn{1}{c|}{} & \multicolumn{1}{c|}{} & \multicolumn{1}{c|}{\cellcolor[HTML]{F8D8D8}N} & \multicolumn{1}{c|}{\cellcolor[HTML]{F8D8D8}-} & \cellcolor[HTML]{F8D8D8}- & \multicolumn{1}{c|}{\cellcolor[HTML]{F8D8D8}43.32} & \multicolumn{1}{c|}{\cellcolor[HTML]{F8D8D8}39.76} & \multicolumn{1}{c|}{\cellcolor[HTML]{F8D8D8}37.01} & \multicolumn{1}{c|}{\cellcolor[HTML]{F8D8D8}35.39} & \multicolumn{1}{c|}{\cellcolor[HTML]{F8D8D8}34.46} & \multicolumn{1}{c|}{\cellcolor[HTML]{F8D8D8}21.56} & \cellcolor[HTML]{F8D8D8}0.1833 \bigstrut \\ \cline{3-12} 
\multicolumn{1}{c|}{} & \multicolumn{1}{c|}{} & \multicolumn{1}{c|}{Y} & \multicolumn{1}{c|}{N} & 0 & \multicolumn{1}{c|}{58.69} & \multicolumn{1}{c|}{58.13} & \multicolumn{1}{c|}{57.62} & \multicolumn{1}{c|}{57.21} & \multicolumn{1}{c|}{56.94} & \multicolumn{1}{c|}{16.8} & 0.3336 \bigstrut \\ \cline{3-12} 
\multicolumn{1}{c|}{} & \multicolumn{1}{c|}{\multirow{-3}{*}{Babbage}} & \multicolumn{1}{c|}{Y} & \multicolumn{1}{c|}{Y} & 0.2 & \multicolumn{1}{c|}{62.79} & \multicolumn{1}{c|}{61.99} & \multicolumn{1}{c|}{61.48} & \multicolumn{1}{c|}{60.85} & \multicolumn{1}{c|}{60.25} & \multicolumn{1}{c|}{12.21} & 0.3327 \bigstrut \\ \clineB{2-12}{2}
\multicolumn{1}{c|}{} & \multicolumn{1}{c|}{} & \multicolumn{1}{c|}{\cellcolor[HTML]{F8D8D8}N} & \multicolumn{1}{c|}{\cellcolor[HTML]{F8D8D8}-} & \cellcolor[HTML]{F8D8D8}- & \multicolumn{1}{c|}{\cellcolor[HTML]{F8D8D8}56.8} & \multicolumn{1}{c|}{\cellcolor[HTML]{F8D8D8}55.61} & \multicolumn{1}{c|}{\cellcolor[HTML]{F8D8D8}53.97} & \multicolumn{1}{c|}{\cellcolor[HTML]{F8D8D8}53.16} & \multicolumn{1}{c|}{\cellcolor[HTML]{F8D8D8}52.17} & \multicolumn{1}{c|}{\cellcolor[HTML]{F8D8D8}19.79} & \cellcolor[HTML]{F8D8D8}0.2507 \bigstrut \\ \cline{3-12} 
\multicolumn{1}{c|}{} & \multicolumn{1}{c|}{} & \multicolumn{1}{c|}{Y} & \multicolumn{1}{c|}{N} & 0 & \multicolumn{1}{c|}{69.97} & \multicolumn{1}{c|}{68.52} & \multicolumn{1}{c|}{67.83} & \multicolumn{1}{c|}{67.42} & \multicolumn{1}{c|}{66.73} & \multicolumn{1}{c|}{10.99} & 0.3461 \bigstrut \\ \cline{3-12} 
\multicolumn{1}{c|}{} & \multicolumn{1}{c|}{\multirow{-3}{*}{Curie}} & \multicolumn{1}{c|}{Y} & \multicolumn{1}{c|}{Y} & 0.2 & \multicolumn{1}{c|}{73.18} & \multicolumn{1}{c|}{72.2} & \multicolumn{1}{c|}{71.18} & \multicolumn{1}{c|}{70.49} & \multicolumn{1}{c|}{69.91} & \multicolumn{1}{c|}{8.92} & 0.355 \bigstrut \\ \clineB{2-12}{2}
\multicolumn{1}{c|}{} & \multicolumn{1}{c|}{} & \multicolumn{1}{c|}{\cellcolor[HTML]{F8D8D8}N} & \multicolumn{1}{c|}{\cellcolor[HTML]{F8D8D8}-} & \cellcolor[HTML]{F8D8D8}- & \multicolumn{1}{c|}{\cellcolor[HTML]{F8D8D8}44.93} & \multicolumn{1}{c|}{\cellcolor[HTML]{F8D8D8}42.11} & \multicolumn{1}{c|}{\cellcolor[HTML]{F8D8D8}40.91} & \multicolumn{1}{c|}{\cellcolor[HTML]{F8D8D8}39.84} & \multicolumn{1}{c|}{\cellcolor[HTML]{F8D8D8}38.99} & \multicolumn{1}{c|}{\cellcolor[HTML]{F8D8D8}11.91} & \cellcolor[HTML]{F8D8D8}0.2247 \bigstrut \\ \cline{3-12} 
\multicolumn{1}{c|}{} & \multicolumn{1}{c|}{} & \multicolumn{1}{c|}{Y} & \multicolumn{1}{c|}{N} & 0 & \multicolumn{1}{c|}{56.69} & \multicolumn{1}{c|}{56.58} & \multicolumn{1}{c|}{56.66} & \multicolumn{1}{c|}{56.47} & \multicolumn{1}{c|}{56.15} & \multicolumn{1}{c|}{15.43} & 0.3397 \bigstrut \\ \cline{3-12} 
\multicolumn{1}{c|}{\multirow{-17}{*}{Codex}} & \multicolumn{1}{c|}{\multirow{-3}{*}{Davinci}} & \multicolumn{1}{c|}{Y} & \multicolumn{1}{c|}{Y} & 0.2 & \multicolumn{1}{c|}{68.07} & \multicolumn{1}{c|}{69.95} & \multicolumn{1}{c|}{67} & \multicolumn{1}{c|}{66.94} & \multicolumn{1}{c|}{66.53} & \multicolumn{1}{c|}{9.47} & 0.3543 \bigstrut \\ \hlineB{2}
\end{tabular}%
}
\end{table*}

\begin{table*}[h]
\centering
\caption{\textbf{Detailed Results of Searching Java Code with Python Code as query}}
\label{tab:python_res}
% \resizebox{\textwidth}{!}
{%
\begin{tabular}{ccccc|ccccccc}
\hlineB{2}
\multicolumn{5}{c|}{\textbf{Settings}} & \multicolumn{7}{c}{\textbf{Metrics}} \bigstrut \\ \hlineB{2}
\multicolumn{1}{c|}{\textbf{Model}} & \multicolumn{1}{c|}{\textbf{Sub-Model}} & \multicolumn{1}{c|}{\textbf{Trained}} & \multicolumn{1}{c|}{\textbf{SSS}} & $\alpha$ & \multicolumn{1}{c|}{\textbf{PR@1}} & \multicolumn{1}{c|}{\textbf{PR@2}} & \multicolumn{1}{c|}{\textbf{PR@3}} & \multicolumn{1}{c|}{\textbf{PR@4}} & \multicolumn{1}{c|}{\textbf{PR@5}} & \multicolumn{1}{c|}{\textbf{AFP}} & \textbf{ARG} \bigstrut \\ \hlineB{2}
\multicolumn{1}{c|}{BM25} & \multicolumn{4}{c|}{\cellcolor[HTML]{FFFFFF}} & \multicolumn{1}{c|}{51.32} & \multicolumn{1}{c|}{50.11} & \multicolumn{1}{c|}{48.98} & \multicolumn{1}{c|}{47.58} & \multicolumn{1}{c|}{46.8} & \multicolumn{1}{c|}{15.33} & 0.2649 \bigstrut \\ \cline{1-1} \cline{6-12} 
\multicolumn{1}{c|}{Token-Subset (COSAL)} & \multicolumn{4}{c|}{\cellcolor[HTML]{FFFFFF}} & \multicolumn{1}{c|}{84.35} & \multicolumn{1}{c|}{82.44} & \multicolumn{1}{c|}{81.09} & \multicolumn{1}{c|}{79.88} & \multicolumn{1}{c|}{79.01} & \multicolumn{1}{c|}{2.15} & 0.3073 \bigstrut \\ \cline{1-1} \cline{6-12} 
\multicolumn{1}{c|}{Tree-Similarity  (stratified)} & \multicolumn{4}{c|}{\multirow{-3}{*}{\cellcolor[HTML]{FFFFFF}No-Training   required}} & \multicolumn{1}{c|}{74.29} & \multicolumn{1}{c|}{71.35} & \multicolumn{1}{c|}{68.56} & \multicolumn{1}{c|}{66.05} & \multicolumn{1}{c|}{65.35} & \multicolumn{1}{c|}{8.56} & 0.2456 \bigstrut \\ \hlineB{2}
\multicolumn{1}{c|}{} & \multicolumn{4}{c|}{CodeBERT  (stratified)} & \multicolumn{1}{c|}{15.5} & \multicolumn{1}{c|}{16.75} & \multicolumn{1}{c|}{17.83} & \multicolumn{1}{c|}{18.38} & \multicolumn{1}{c|}{18.1} & \multicolumn{1}{c|}{130.33} & 0.2248 \bigstrut \\ \cline{2-12} 
\multicolumn{1}{c|}{} & \multicolumn{4}{c|}{GraphCodeBERT    (stratified)} & \multicolumn{1}{c|}{20.5} & \multicolumn{1}{c|}{21} & \multicolumn{1}{c|}{21.83} & \multicolumn{1}{c|}{22.25} & \multicolumn{1}{c|}{22.7} & \multicolumn{1}{c|}{142.85} & 0.2099 \bigstrut \\ \cline{2-12} 
\multicolumn{1}{c|}{\multirow{-3}{*}{Single-Encoder   Models}} & \multicolumn{4}{c|}{UnixCoder  (stratified)} & \multicolumn{1}{c|}{25} & \multicolumn{1}{c|}{25.25} & \multicolumn{1}{c|}{25.17} & \multicolumn{1}{c|}{25.88} & \multicolumn{1}{c|}{25.9} & \multicolumn{1}{c|}{57.5} & 0.3553 \bigstrut \\ \hlineB{2}
\multicolumn{1}{c|}{} & \multicolumn{1}{c|}{\cellcolor[HTML]{F8D8D8}-} & \multicolumn{1}{c|}{\cellcolor[HTML]{F8D8D8}N} & \multicolumn{1}{c|}{\cellcolor[HTML]{F8D8D8}-} & \cellcolor[HTML]{F8D8D8}- & \multicolumn{1}{c|}{\cellcolor[HTML]{F8D8D8}9.01} & \multicolumn{1}{c|}{\cellcolor[HTML]{F8D8D8}8.57} & \multicolumn{1}{c|}{\cellcolor[HTML]{F8D8D8}8.96} & \multicolumn{1}{c|}{\cellcolor[HTML]{F8D8D8}9.18} & \multicolumn{1}{c|}{\cellcolor[HTML]{F8D8D8}9.02} & \multicolumn{1}{c|}{\cellcolor[HTML]{F8D8D8}48.58} & \cellcolor[HTML]{F8D8D8}0.0875 \bigstrut \\ \cline{2-12} 
\multicolumn{1}{c|}{} & \multicolumn{1}{c|}{\cellcolor[HTML]{FCE5CD}-} & \multicolumn{1}{c|}{\cellcolor[HTML]{FCE5CD}Y} & \multicolumn{1}{c|}{\cellcolor[HTML]{FCE5CD}N} & \cellcolor[HTML]{FCE5CD}0 & \multicolumn{1}{c|}{\cellcolor[HTML]{FCE5CD}89.75} & \multicolumn{1}{c|}{\cellcolor[HTML]{FCE5CD}87.48} & \multicolumn{1}{c|}{\cellcolor[HTML]{FCE5CD}86.75} & \multicolumn{1}{c|}{\cellcolor[HTML]{FCE5CD}85.44} & \multicolumn{1}{c|}{\cellcolor[HTML]{FCE5CD}84.62} & \multicolumn{1}{c|}{\cellcolor[HTML]{FCE5CD}3.424} & \cellcolor[HTML]{FCE5CD}0.392 \bigstrut \\ \cline{2-12} 
\multicolumn{1}{c|}{\multirow{-3}{*}{CodeBERT }} & \multicolumn{1}{c|}{\cellcolor[HTML]{D9EAD3}{\color[HTML]{00009B} \textbf{-}}} & \multicolumn{1}{c|}{\cellcolor[HTML]{D9EAD3}{\color[HTML]{00009B} \textbf{Y}}} & \multicolumn{1}{c|}{\cellcolor[HTML]{D9EAD3}{\color[HTML]{00009B} \textbf{Y}}} & \cellcolor[HTML]{D9EAD3}{\color[HTML]{00009B} \textbf{0.2}} & \multicolumn{1}{c|}{\cellcolor[HTML]{00FF00}{\color[HTML]{00009B} \textbf{94.05}}} & \multicolumn{1}{c|}{\cellcolor[HTML]{00FF00}{\color[HTML]{00009B} \textbf{92.98}}} & \multicolumn{1}{c|}{\cellcolor[HTML]{00FF00}{\color[HTML]{00009B} \textbf{92.01}}} & \multicolumn{1}{c|}{\cellcolor[HTML]{00FF00}{\color[HTML]{00009B} \textbf{91.11}}} & \multicolumn{1}{c|}{\cellcolor[HTML]{00FF00}{\color[HTML]{00009B} \textbf{90.37}}} & \multicolumn{1}{c|}{\cellcolor[HTML]{00FF00}{\color[HTML]{00009B} \textbf{3.64}}} & \cellcolor[HTML]{00FF00}{\color[HTML]{00009B} \textbf{0.4051}} \bigstrut \\ \hlineB{2}
\multicolumn{1}{c|}{} & \multicolumn{1}{c|}{} & \multicolumn{1}{c|}{\cellcolor[HTML]{F8D8D8}N} & \multicolumn{1}{c|}{\cellcolor[HTML]{F8D8D8}-} & \cellcolor[HTML]{F8D8D8}- & \multicolumn{1}{c|}{\cellcolor[HTML]{F8D8D8}78.15} & \multicolumn{1}{c|}{\cellcolor[HTML]{F8D8D8}76.19} & \multicolumn{1}{c|}{\cellcolor[HTML]{F8D8D8}74.39} & \multicolumn{1}{c|}{\cellcolor[HTML]{F8D8D8}73.14} & \multicolumn{1}{c|}{\cellcolor[HTML]{F8D8D8}71.93} & \multicolumn{1}{c|}{\cellcolor[HTML]{F8D8D8}3.91} & \cellcolor[HTML]{F8D8D8}0.2378 \bigstrut \\ \cline{3-12} 
\multicolumn{1}{c|}{} & \multicolumn{1}{c|}{} & \multicolumn{1}{c|}{Y} & \multicolumn{1}{c|}{N} & 0 & \multicolumn{1}{c|}{83.97} & \multicolumn{1}{c|}{83.69} & \multicolumn{1}{c|}{82.94} & \multicolumn{1}{c|}{81.64} & \multicolumn{1}{c|}{80.89} & \multicolumn{1}{c|}{3.57} & 0.404 \bigstrut \\ \cline{3-12} 
\multicolumn{1}{c|}{} & \multicolumn{1}{c|}{\multirow{-3}{*}{Ada}} & \multicolumn{1}{c|}{Y} & \multicolumn{1}{c|}{Y} & 0.2 & \multicolumn{1}{c|}{87.88} & \multicolumn{1}{c|}{87.14} & \multicolumn{1}{c|}{86.45} & \multicolumn{1}{c|}{86.08} & \multicolumn{1}{c|}{85.45} & \multicolumn{1}{c|}{2.71} & 0.4037 \bigstrut \\ \clineB{2-12}{2} 
\multicolumn{1}{c|}{} & \multicolumn{1}{c|}{} & \multicolumn{1}{c|}{\cellcolor[HTML]{F8D8D8}N} & \multicolumn{1}{c|}{\cellcolor[HTML]{F8D8D8}-} & \cellcolor[HTML]{F8D8D8}- & \multicolumn{1}{c|}{\cellcolor[HTML]{F8D8D8}76.36} & \multicolumn{1}{c|}{\cellcolor[HTML]{F8D8D8}74.62} & \multicolumn{1}{c|}{\cellcolor[HTML]{F8D8D8}72.97} & \multicolumn{1}{c|}{\cellcolor[HTML]{F8D8D8}71.56} & \multicolumn{1}{c|}{\cellcolor[HTML]{F8D8D8}70.36} & \multicolumn{1}{c|}{\cellcolor[HTML]{F8D8D8}3.68} & \cellcolor[HTML]{F8D8D8}0.2395 \bigstrut \\ \cline{3-12} 
\multicolumn{1}{c|}{} & \multicolumn{1}{c|}{} & \multicolumn{1}{c|}{Y} & \multicolumn{1}{c|}{N} & 0 & \multicolumn{1}{c|}{80.31} & \multicolumn{1}{c|}{78.78} & \multicolumn{1}{c|}{78.3} & \multicolumn{1}{c|}{77.56} & \multicolumn{1}{c|}{76.99} & \multicolumn{1}{c|}{3.88} & 0.3986 \bigstrut \\ \cline{3-12} 
\multicolumn{1}{c|}{} & \multicolumn{1}{c|}{\multirow{-3}{*}{Babbage}} & \multicolumn{1}{c|}{Y} & \multicolumn{1}{c|}{Y} & 0.2 & \multicolumn{1}{c|}{82.23} & \multicolumn{1}{c|}{80.23} & \multicolumn{1}{c|}{79.25} & \multicolumn{1}{c|}{78.21} & \multicolumn{1}{c|}{77.2} & \multicolumn{1}{c|}{3.32} & 0.3917 \bigstrut \\ \clineB{2-12}{2} 
\multicolumn{1}{c|}{} & \multicolumn{1}{c|}{} & \multicolumn{1}{c|}{\cellcolor[HTML]{F8D8D8}N} & \multicolumn{1}{c|}{\cellcolor[HTML]{F8D8D8}-} & \cellcolor[HTML]{F8D8D8}- & \multicolumn{1}{c|}{\cellcolor[HTML]{F8D8D8}75.89} & \multicolumn{1}{c|}{\cellcolor[HTML]{F8D8D8}74.38} & \multicolumn{1}{c|}{\cellcolor[HTML]{F8D8D8}73.44} & \multicolumn{1}{c|}{\cellcolor[HTML]{F8D8D8}71.9} & \multicolumn{1}{c|}{\cellcolor[HTML]{F8D8D8}70.82} & \multicolumn{1}{c|}{\cellcolor[HTML]{F8D8D8}11.44} & \cellcolor[HTML]{F8D8D8}0.23 \bigstrut \\ \cline{3-12} 
\multicolumn{1}{c|}{} & \multicolumn{1}{c|}{} & \multicolumn{1}{c|}{Y} & \multicolumn{1}{c|}{N} & 0 & \multicolumn{1}{c|}{82.14} & \multicolumn{1}{c|}{81.85} & \multicolumn{1}{c|}{81.29} & \multicolumn{1}{c|}{80.72} & \multicolumn{1}{c|}{80.19} & \multicolumn{1}{c|}{3.29} & 0.4081 \bigstrut \\ \cline{3-12} 
\multicolumn{1}{c|}{} & \multicolumn{1}{c|}{\multirow{-3}{*}{Curie}} & \multicolumn{1}{c|}{Y} & \multicolumn{1}{c|}{Y} & 0.2 & \multicolumn{1}{c|}{88.44} & \multicolumn{1}{c|}{87.56} & \multicolumn{1}{c|}{86.78} & \multicolumn{1}{c|}{85.69} & \multicolumn{1}{c|}{84.93} & \multicolumn{1}{c|}{2.93} & 0.4112 \bigstrut \\ \clineB{2-12}{2} 
\multicolumn{1}{c|}{} & \multicolumn{1}{c|}{} & \multicolumn{1}{c|}{\cellcolor[HTML]{F8D8D8}N} & \multicolumn{1}{c|}{\cellcolor[HTML]{F8D8D8}-} & \cellcolor[HTML]{F8D8D8}- & \multicolumn{1}{c|}{\cellcolor[HTML]{F8D8D8}45.2} & \multicolumn{1}{c|}{\cellcolor[HTML]{F8D8D8}44.66} & \multicolumn{1}{c|}{\cellcolor[HTML]{F8D8D8}43.13} & \multicolumn{1}{c|}{\cellcolor[HTML]{F8D8D8}42.09} & \multicolumn{1}{c|}{\cellcolor[HTML]{F8D8D8}41.05} & \multicolumn{1}{c|}{\cellcolor[HTML]{F8D8D8}10.03} & \cellcolor[HTML]{F8D8D8}0.2082 \bigstrut \\ \cline{3-12} 
\multicolumn{1}{c|}{} & \multicolumn{1}{c|}{} & \multicolumn{1}{c|}{Y} & \multicolumn{1}{c|}{N} & 0 & \multicolumn{1}{c|}{68.11} & \multicolumn{1}{c|}{68.26} & \multicolumn{1}{c|}{67.9} & \multicolumn{1}{c|}{67.28} & \multicolumn{1}{c|}{66.96} & \multicolumn{1}{c|}{4.85} & 0.3799 \bigstrut \\ \cline{3-12} 
\multicolumn{1}{c|}{\multirow{-12}{*}{Codex}} & \multicolumn{1}{c|}{\multirow{-3}{*}{Davinci}} & \multicolumn{1}{c|}{Y} & \multicolumn{1}{c|}{Y} & 0.2 & \multicolumn{1}{c|}{81.89} & \multicolumn{1}{c|}{81.1} & \multicolumn{1}{c|}{80.12} & \multicolumn{1}{c|}{79.52} & \multicolumn{1}{c|}{78.72} & \multicolumn{1}{c|}{3.59} & 0.3986 \bigstrut \\ \hlineB{2}
\end{tabular}%
}
\end{table*}

\begin{table*}[h]
\caption{\textbf{Impact of Positive and Negative samples. Max-p and Max-n stand for Maximum Positive samples and Maximum Negative samples, respectively.}}
\label{tab:impact}
\resizebox{\textwidth}{!}{%
\begin{tabular}{c|cc||ccccccc||ccccccc}
\hlineB{2}
 &  &  & \multicolumn{7}{c||}{\textbf{Java}} & \multicolumn{7}{c}{\textbf{Python}} \bigstrut \\ \cline{4-17} 
\multirow{-2}{*}{\textbf{Model}} & \multirow{-2}{*}{\textbf{Max-p}} & \multirow{-2}{*}{\textbf{Max-N}} & \multicolumn{1}{c|}{\textbf{PR@1}} & \multicolumn{1}{c|}{\textbf{PR@2}} & \multicolumn{1}{c|}{\textbf{PR@3}} & \multicolumn{1}{c|}{\textbf{PR@4}} & \multicolumn{1}{c|}{\textbf{PR@5}} & \multicolumn{1}{c|}{\textbf{AFP}} & \textbf{ARG} & \multicolumn{1}{c|}{\textbf{PR@1}} & \multicolumn{1}{c|}{\textbf{PR@2}} & \multicolumn{1}{c|}{\textbf{PR@3}} & \multicolumn{1}{c|}{\textbf{PR@4}} & \multicolumn{1}{c|}{\textbf{PR@5}} & \multicolumn{1}{c|}{\textbf{AFP}} & \textbf{ARG} \bigstrut \\ \hlineB{2}
 & 5 & 5 & \multicolumn{1}{c|}{{ 86.47}} & \multicolumn{1}{c|}{{ 85.46}} & \multicolumn{1}{c|}{{ 84.77}} & \multicolumn{1}{c|}{{ 83.77}} & \multicolumn{1}{c|}{{ 82.62}} & \multicolumn{1}{c|}{{ 9.53}} & { 0.3857} & \multicolumn{1}{c|}{{ 94.05}} & \multicolumn{1}{c|}{{ 92.98}} & \multicolumn{1}{c|}{{ 92.01}} & \multicolumn{1}{c|}{{ 91.11}} & \multicolumn{1}{c|}{{ 90.37}} & \multicolumn{1}{c|}{{ 3.64}} & { 0.4051} \bigstrut \\ 
 & 5 & 0 & \multicolumn{1}{c|}{7.06} & \multicolumn{1}{c|}{7.06} & \multicolumn{1}{c|}{7.06} & \multicolumn{1}{c|}{7.06} & \multicolumn{1}{c|}{7.06} & \multicolumn{1}{c|}{215.26} & 0.0101 & \multicolumn{1}{c|}{5.29} & \multicolumn{1}{c|}{8.59} & \multicolumn{1}{c|}{7.19} & \multicolumn{1}{c|}{4.46} & \multicolumn{1}{c|}{7.08} & \multicolumn{1}{c|}{50.38} & 0.0476 \bigstrut \\ 
 & 0 & 5 & \multicolumn{1}{c|}{5.58} & \multicolumn{1}{c|}{4.24} & \multicolumn{1}{c|}{4.67} & \multicolumn{1}{c|}{4.82} & \multicolumn{1}{c|}{4.56} & \multicolumn{1}{c|}{150.72} & 0.0111 & \multicolumn{1}{c|}{8.84} & \multicolumn{1}{c|}{7.29} & \multicolumn{1}{c|}{5.75} & \multicolumn{1}{c|}{5.91} & \multicolumn{1}{c|}{5.4} & \multicolumn{1}{c|}{76.93} & -0.0109 \bigstrut \\ 
 & 1 & 1 & \multicolumn{1}{c|}{82.02} & \multicolumn{1}{c|}{81.6} & \multicolumn{1}{c|}{80.71} & \multicolumn{1}{c|}{79.94} & \multicolumn{1}{c|}{79.06} & \multicolumn{1}{c|}{9.82} & 0.3461 & \multicolumn{1}{c|}{93.41} & \multicolumn{1}{c|}{93} & \multicolumn{1}{c|}{92.36} & \multicolumn{1}{c|}{91.64} & \multicolumn{1}{c|}{91.04} & \multicolumn{1}{c|}{2.5} & 0.418 \bigstrut \\ 
\multirow{-7}{*}{\textbf{CodeBERT}} & 3 & 3 & \multicolumn{1}{c|}{83.5} & \multicolumn{1}{c|}{82.52} & \multicolumn{1}{c|}{81.58} & \multicolumn{1}{c|}{80.83} & \multicolumn{1}{c|}{79.88} & \multicolumn{1}{c|}{10.99} & 0.3612 & \multicolumn{1}{c|}{94.26} & \multicolumn{1}{c|}{93.13} & \multicolumn{1}{c|}{92.55} & \multicolumn{1}{c|}{91.78} & \multicolumn{1}{c|}{91.22} & \multicolumn{1}{c|}{2.45} & 0.3918 \bigstrut \\ \hlineB{2}
 & 5 & 5 & \multicolumn{1}{c|}{66.77} & \multicolumn{1}{c|}{65.85} & \multicolumn{1}{c|}{65.24} & \multicolumn{1}{c|}{64.58} & \multicolumn{1}{c|}{63.81} & \multicolumn{1}{c|}{10.6} & 0.3458 & \multicolumn{1}{c|}{87.88} & \multicolumn{1}{c|}{87.14} & \multicolumn{1}{c|}{86.45} & \multicolumn{1}{c|}{86.08} & \multicolumn{1}{c|}{85.45} & \multicolumn{1}{c|}{2.71} & 0.4037 \bigstrut \\ 
 & 5 & 0 & \multicolumn{1}{c|}{14.12} & \multicolumn{1}{c|}{15.85} & \multicolumn{1}{c|}{15.98} & \multicolumn{1}{c|}{15.98} & \multicolumn{1}{c|}{16.1} & \multicolumn{1}{c|}{76.73} & 0.087 & \multicolumn{1}{c|}{7.53} & \multicolumn{1}{c|}{9.2} & \multicolumn{1}{c|}{9.67} & \multicolumn{1}{c|}{9.92} & \multicolumn{1}{c|}{9.95} & \multicolumn{1}{c|}{39.85} & 0.1263 \bigstrut \\ 
 & 0 & 5 & \multicolumn{1}{c|}{5.46} & \multicolumn{1}{c|}{4.51} & \multicolumn{1}{c|}{4.69} & \multicolumn{1}{c|}{5.14} & \multicolumn{1}{c|}{5.61} & \multicolumn{1}{c|}{65.23} & 0.0342 & \multicolumn{1}{c|}{0} & \multicolumn{1}{c|}{0.74} & \multicolumn{1}{c|}{1.59} & \multicolumn{1}{c|}{1.76} & \multicolumn{1}{c|}{1.98} & \multicolumn{1}{c|}{58.13} & 0.0407 \bigstrut \\ 
 & 1 & 1 & \multicolumn{1}{c|}{63.62} & \multicolumn{1}{c|}{62.08} & \multicolumn{1}{c|}{61.09} & \multicolumn{1}{c|}{60.06} & \multicolumn{1}{c|}{59.41} & \multicolumn{1}{c|}{15.98} & 0.326 & \multicolumn{1}{c|}{85.33} & \multicolumn{1}{c|}{84.59} & \multicolumn{1}{c|}{84.35} & \multicolumn{1}{c|}{83.44} & \multicolumn{1}{c|}{82.74} & \multicolumn{1}{c|}{2.46} & 0.3967 \bigstrut \\ 
\multirow{-7}{*}{\textbf{Ada}} & 3 & 3 & \multicolumn{1}{c|}{66.88} & \multicolumn{1}{c|}{64.84} & \multicolumn{1}{c|}{64.47} & \multicolumn{1}{c|}{63.34} & \multicolumn{1}{c|}{32.62} & \multicolumn{1}{c|}{12.21} & 0.3462 & \multicolumn{1}{c|}{87.29} & \multicolumn{1}{c|}{86.05} & \multicolumn{1}{c|}{85.25} & \multicolumn{1}{c|}{84.48} & \multicolumn{1}{c|}{83.95} & \multicolumn{1}{c|}{3.26} & 0.4024 \bigstrut \\ \hlineB{2}
 & 5 & 5 & \multicolumn{1}{c|}{62.79} & \multicolumn{1}{c|}{61.99} & \multicolumn{1}{c|}{61.48} & \multicolumn{1}{c|}{60.85} & \multicolumn{1}{c|}{60.25} & \multicolumn{1}{c|}{12.21} & 0.3327 & \multicolumn{1}{c|}{82.23} & \multicolumn{1}{c|}{80.23} & \multicolumn{1}{c|}{79.25} & \multicolumn{1}{c|}{78.21} & \multicolumn{1}{c|}{77.2} & \multicolumn{1}{c|}{3.32} & 0.3917 \bigstrut \\ 
 & 5 & 0 & \multicolumn{1}{c|}{20.59} & \multicolumn{1}{c|}{19.7} & \multicolumn{1}{c|}{17.94} & \multicolumn{1}{c|}{16.91} & \multicolumn{1}{c|}{16.22} & \multicolumn{1}{c|}{40.42} & 0.0951 & \multicolumn{1}{c|}{8.21} & \multicolumn{1}{c|}{8.25} & \multicolumn{1}{c|}{7.36} & \multicolumn{1}{c|}{7.38} & \multicolumn{1}{c|}{6.79} & \multicolumn{1}{c|}{39.12} & 0.0932 \bigstrut \\ 
 & 0 & 5 & \multicolumn{1}{c|}{3.98} & \multicolumn{1}{c|}{4.07} & \multicolumn{1}{c|}{4.41} & \multicolumn{1}{c|}{3.95} & \multicolumn{1}{c|}{4.26} & \multicolumn{1}{c|}{52.47} & 0.0331 & \multicolumn{1}{c|}{2.76} & \multicolumn{1}{c|}{3.19} & \multicolumn{1}{c|}{3.1} & \multicolumn{1}{c|}{3.89} & \multicolumn{1}{c|}{4.12} & \multicolumn{1}{c|}{49.13} & -0.0062 \bigstrut \\ 
 & 1 & 1 & \multicolumn{1}{c|}{57.27} & \multicolumn{1}{c|}{56.11} & \multicolumn{1}{c|}{55.21} & \multicolumn{1}{c|}{54.72} & \multicolumn{1}{c|}{53.97} & \multicolumn{1}{c|}{17.2} & 0.3115 & \multicolumn{1}{c|}{79.21} & \multicolumn{1}{c|}{77.95} & \multicolumn{1}{c|}{76.7} & \multicolumn{1}{c|}{75.67} & \multicolumn{1}{c|}{74.82} & \multicolumn{1}{c|}{3.003} & 0.384 \bigstrut \\ 
\multirow{-7}{*}{\textbf{Babbage}} & 3 & 3 & \multicolumn{1}{c|}{64.45} & \multicolumn{1}{c|}{62.88} & \multicolumn{1}{c|}{61.72} & \multicolumn{1}{c|}{60.79} & \multicolumn{1}{c|}{59.7} & \multicolumn{1}{c|}{11.84} & 0.3354 & \multicolumn{1}{c|}{80.95} & \multicolumn{1}{c|}{79.87} & \multicolumn{1}{c|}{78.81} & \multicolumn{1}{c|}{77.71} & \multicolumn{1}{c|}{76.9} & \multicolumn{1}{c|}{3.04} & 0.3916 \bigstrut \\ \hlineB{2}
 & 5 & 5 & \multicolumn{1}{c|}{73.18} & \multicolumn{1}{c|}{72.2} & \multicolumn{1}{c|}{71.18} & \multicolumn{1}{c|}{70.49} & \multicolumn{1}{c|}{69.91} & \multicolumn{1}{c|}{8.92} & 0.355 & \multicolumn{1}{c|}{88.44} & \multicolumn{1}{c|}{87.56} & \multicolumn{1}{c|}{86.78} & \multicolumn{1}{c|}{85.69} & \multicolumn{1}{c|}{84.93} & \multicolumn{1}{c|}{2.93} & 0.4112 \bigstrut \\ 
 & 5 & 0 & \multicolumn{1}{c|}{9.55} & \multicolumn{1}{c|}{13.74} & \multicolumn{1}{c|}{13.93} & \multicolumn{1}{c|}{13.72} & \multicolumn{1}{c|}{13.78} & \multicolumn{1}{c|}{44.02} & 0.11 & \multicolumn{1}{c|}{17.18} & \multicolumn{1}{c|}{16.65} & \multicolumn{1}{c|}{14.6} & \multicolumn{1}{c|}{12.76} & \multicolumn{1}{c|}{11.53} & \multicolumn{1}{c|}{49.28} & 0.0869 \bigstrut \\ 
 & 0 & 5 & \multicolumn{1}{c|}{5.52} & \multicolumn{1}{c|}{4.27} & \multicolumn{1}{c|}{3.26} & \multicolumn{1}{c|}{2.66} & \multicolumn{1}{c|}{3.78} & \multicolumn{1}{c|}{81.7674} & 0.0261 & \multicolumn{1}{c|}{1.32} & \multicolumn{1}{c|}{2.47} & \multicolumn{1}{c|}{3.26} & \multicolumn{1}{c|}{3.35} & \multicolumn{1}{c|}{3.31} & \multicolumn{1}{c|}{40.11} & 0.0051 \bigstrut \\ 
 & 1 & 1 & \multicolumn{1}{c|}{62.85} & \multicolumn{1}{c|}{62.76} & \multicolumn{1}{c|}{62.81} & \multicolumn{1}{c|}{62.3} & \multicolumn{1}{c|}{61.73} & \multicolumn{1}{c|}{12.02} & 0.3384 & \multicolumn{1}{c|}{82.48} & \multicolumn{1}{c|}{81.19} & \multicolumn{1}{c|}{80.1} & \multicolumn{1}{c|}{79.29} & \multicolumn{1}{c|}{78.57} & \multicolumn{1}{c|}{3.09} & 0.391 \bigstrut \\ 
\multirow{-7}{*}{\textbf{Curie}} & 3 & 3 & \multicolumn{1}{c|}{71.93} & \multicolumn{1}{c|}{70.5} & \multicolumn{1}{c|}{70.07} & \multicolumn{1}{c|}{69.36} & \multicolumn{1}{c|}{68.74} & \multicolumn{1}{c|}{11.26} & 0.3496 & \multicolumn{1}{c|}{87.5} & \multicolumn{1}{c|}{86.61} & \multicolumn{1}{c|}{86.18} & \multicolumn{1}{c|}{85.52} & \multicolumn{1}{c|}{84.89} & \multicolumn{1}{c|}{3.11} & 0.4059 \bigstrut \\ \hlineB{2}
 & 5 & 5 & \multicolumn{1}{c|}{68.07} & \multicolumn{1}{c|}{69.95} & \multicolumn{1}{c|}{67} & \multicolumn{1}{c|}{66.94} & \multicolumn{1}{c|}{66.53} & \multicolumn{1}{c|}{9.47} & 0.3543 & \multicolumn{1}{c|}{81.89} & \multicolumn{1}{c|}{81.1} & \multicolumn{1}{c|}{80.12} & \multicolumn{1}{c|}{79.52} & \multicolumn{1}{c|}{78.72} & \multicolumn{1}{c|}{3.59} & 0.3986 \bigstrut \\ 
 & 5 & 0 & \multicolumn{1}{c|}{3.5} & \multicolumn{1}{c|}{2.82} & \multicolumn{1}{c|}{3.72} & \multicolumn{1}{c|}{4.42} & \multicolumn{1}{c|}{5.08} & \multicolumn{1}{c|}{45.42} & 0.0468 & \multicolumn{1}{c|}{6.25} & \multicolumn{1}{c|}{6.25} & \multicolumn{1}{c|}{5.8} & \multicolumn{1}{c|}{5.68} & \multicolumn{1}{c|}{5.86} & \multicolumn{1}{c|}{49.86} & 0.0405 \bigstrut \\ 
 & 0 & 5 & \multicolumn{1}{c|}{3.98} & \multicolumn{1}{c|}{6.32} & \multicolumn{1}{c|}{4.79} & \multicolumn{1}{c|}{3.83} & \multicolumn{1}{c|}{3.65} & \multicolumn{1}{c|}{70.43} & 0.0011 & \multicolumn{1}{c|}{1.49} & \multicolumn{1}{c|}{0.87} & \multicolumn{1}{c|}{1.09} & \multicolumn{1}{c|}{0.84} & \multicolumn{1}{c|}{1.22} & \multicolumn{1}{c|}{46.26} & -0.0145 \bigstrut \\ 
 & 1 & 1 & \multicolumn{1}{c|}{41.13} & \multicolumn{1}{c|}{41.69} & \multicolumn{1}{c|}{42.02} & \multicolumn{1}{c|}{41.97} & \multicolumn{1}{c|}{41.73} & \multicolumn{1}{c|}{15.6} & 0.3218 & \multicolumn{1}{c|}{51.87} & \multicolumn{1}{c|}{50.83} & \multicolumn{1}{c|}{50.11} & \multicolumn{1}{c|}{50.05} & \multicolumn{1}{c|}{49.26} & \multicolumn{1}{c|}{6.61} & 0.3699 \bigstrut \\ 
\multirow{-7}{*}{\textbf{Davinci}} & 3 & 3 & \multicolumn{1}{c|}{62.91} & \multicolumn{1}{c|}{62.88} & \multicolumn{1}{c|}{62.51} & \multicolumn{1}{c|}{61.77} & \multicolumn{1}{c|}{61.19} & \multicolumn{1}{c|}{8.83} & 0.3452 & \multicolumn{1}{c|}{69.05} & \multicolumn{1}{c|}{68.75} & \multicolumn{1}{c|}{68.3} & \multicolumn{1}{c|}{67.92} & \multicolumn{1}{c|}{67.3} & \multicolumn{1}{c|}{5.22} & 0.3929 \bigstrut \\ \hlineB{2}
\end{tabular}%
}
\end{table*}
